# Supplementary material for: Gloss-Free End-to-End Sign Language Translation
Source: arXiv:2305.12876 source file (2023-05-27)
Supplement: Supplementary file 1 [file appendix.tex]

\appendix

\section{Appendix}
\label{sec:appendix}

\subsection{Results on PHOENIX14\textbf{T}}

\textbf{PHOENIX2014-T}: PHOENIX14\textbf{T}\cite{camgoz2018neural} is a German sign language dataset that contains parallel corpus including sign language videos, gloss annotations and spoken German translations. It consists of $8257$ sample of weather and news clips which is then split into Train, Dev and Test subsets with $7096$, $519$ and $642$ samples respectively. 

\subsection{Details about pose extraction}

\subsection{Effects of parameter $\mu$}
